# Supplementary material for: Interplay of spin-dependent delocalization and magnetic anisotropy in the ground and excited states of [Gd$_2$@C$_{78}$]$^{-1}$ and [Gd$_2$@C$_{80}$]$^{-1}$
Source: arXiv:1802.09068 source file (2018-02-25)
Supplement: Supplementary file 1 [file supplementary_material.pdf]

Supplementary material for

# Interplay of spin-dependent delocalization and magnetic anisotropy in the ground and excited states of $[Gd_2@C_{78}]^-$ and $[Gd_2@C_{80}]^-$

Akseli Mansikkamäki,[1,2,a] Alexey A. Popov,[3] Qingming Deng,[3,4] Naoya Iwahara,[1] and Liviu F. Chibotaru[1,b]

[1] *Theory of Nanomaterials Group, Chemistry Department, Katholieke Universiteit Leuven, Celestijnenlaan 200F, 3001 Leuven, Belgium.*

[2] *Department of Chemistry, Nanoscience Center, University of Jyväskylä, P. O. Box 35, Jyväskylä, FI-40014, Finland.*

[3] *Leibniz Institute for Solid State and Materials Research Dresden, Helmholtzstrasse 20, Dresden 01069, Germany.*

[4] *School of Physics and Electronic Electrical Engineering, Huaiyin Normal University, Huai'an, 223001, China.*

[a] Electronic mail: akseli.mansikkamaki@jyu.fi

[b] Electronic mail: liviu.chibotaru@chem.kuleuven.be

CONTENTS

**I. Geometry optimizations** 3

**II. Energies of the exchange states in the ground Σ manifold** 4

A. Eigenvalues of the three-site exchange Hamiltonian 4

B. Extraction of exchange coupling constants from broken symmetry DFT calculations 4

C. Calculation of zero-field splitting parameters 5

**III. Derivations** 8

A. Matrix elements of the free-ion Hamiltonian 8

B. Matrix elements of the single-ion Hamiltonians for a $4f^7 5d^1$ configuration 10

C. Matrix elements of the transfer Hamiltonian for Π and Δ 5d states 12

D. Matrix elements of the transfer Hamiltonian for 4f configurations 14

**IV. Additional figures** 17

**V. Additional tables** 20

**VI. Optimized Cartesian coordinates of 1 and 2** 28

**References** 34

# I. GEOMETRY OPTIMIZATIONS

Before proceeding to the structural optimization of Gd-EMFs $[Gd_2@C_{78}]^-$ (**1**) and $[Gd_2@C_{80}]^-$ (**2**), preliminary calculations were performed for the respective $[Y_2@C_{78}]^-$ and $[Y_2@C_{80}]^-$ analogs at PBE[1,2] level. Original TZ2P-quality 6,3,2/11,6,2 basis set was used for carbon and SBK-type effective core potential with 5,5,4/9,9,8 valence part was used for Y as implemented in Priroda code.[3] Interior of fullerene cages, especially those of highly symmetrical ones, is rather uniform, which results in the possibility of several low-energy configuration of metal ions inside the cage. To clarify possible structure of dimetallofullerene anions, we first performed calculations for $[Y_2@C_{78}]^-$ and $[Y_2@C_{80}\text{-}I_h]^-$ anions with different orientation of $[Y_2]^{n+}$ dimers inside the cage.

Elongated $C_{78}\text{-}D_{3h}(5)$ cage is known for several types of EMFs. In dimetallofullerenes $La_2@C_{78}$[4] and $Ce_2@C_{78}$[5] metal ions are believed to be located close to the poles, which maximizes the metal-metal distance. In nitride clusterfullerene $Sc_3N@C_{78}$,[6] the metal ions are coordinated to the equator of the cage. In $Ti_2C_2@C_{78}$[7,8] and $Ti_2S@C_{78}$,[9] DFT calculations also predicted coordination of Ti atoms to the poles of the cage. For $[Y_2@C_{78}]^-$, our calculation predicts that the structure with Y ions near the poles is at least $90\,\mathrm{kJ\,mol^{-1}}$ lower in energy than the structures with metal ions near the equator (three such isomers with somewhat different positions of metal ions near equator were found). The two lowest energy isomers were then chosen as the starting points for the optimization of **1** and gave an energy difference of $93.4\,\mathrm{kJ\,mol^{-1}}$ in favor of the pole-coordinated isomer of **1**. The latter isomer was then studied throughout the work.

In the case of $[Y_2@C_{80}\text{-}I_h]^-$, calculations started from five different positions of the $[Y_2]^{n+}$ dimer converged to two unique minima with an energy difference of $16.4\,\mathrm{kJ\,mol^{-1}}$. In the most stable geometry, metal atoms have $\eta^6$ coordination to the cage hexagons, resulting in the overall $D_{2h}$ symmetry. In the less stable configuration, Y ions are located close to the pentagon/hexagon edges in quasi-$\eta^2$ fashion, resulting in an overall $C_s$ symmetry of the molecule. These configurations were used as starting points for optimization of corresponding isomers of **2**. In the course of the optimization, both structures converged to the same minimum with a $D_{2h}$ symmetry and $\eta^6$ coordination of Gd ions to the cage hexagons.

## II. ENERGIES OF THE EXCHANGE STATES IN THE GROUND $\Sigma$ MANIFOLD

### A. Eigenvalues of the three-site exchange Hamiltonian

The three-site Hamiltonian describing the exchange interactions in the ground $\Sigma$ manifold is of the form

$$\hat{H}_{\text{3-site}} = -J_{\text{Gd}-\text{Gd}}\hat{\mathbf{S}}_{0,a} \cdot \hat{\mathbf{S}}_{0,b} - J_{\text{Gd}-5\text{d}} \left( \hat{\mathbf{s}} \cdot \hat{\mathbf{S}}_{0,a} + \hat{\mathbf{s}} \cdot \hat{\mathbf{S}}_{0,b} \right), \tag{1}$$

where $\hat{\mathbf{S}}_{0,a}$ and $\hat{\mathbf{S}}_{0,b}$ act on the $S_0 = 7/2$ spins of the 4f electrons at Gd ion $a$ and $b$, respectively, and $\hat{\mathbf{s}}$ acts on the spin of the 5d electron. The two exchange coupling constants, $J_{\text{Gd}-\text{Gd}}$ and $J_{\text{Gd}-5\text{d}}$, describe the exchange interaction between the total 4f spins of the two Gd ions and the Hund's rule -like exchange interaction between the total 4f spins and the spin of the 5d electron, respectively. In order to construct the spectrum of the exchange states in the ground $\Sigma$ manifold from the values of the exchange coupling constants, the Hamiltonian must be diagonalized. This procedure has been discussed by Kahn[10] and the eigenvalues are

$$E(S, S_{\text{core}}) = -\frac{1}{2} J_{\text{Gd}-5\text{d}} S(S+1) - \frac{1}{2}(J_{\text{Gd}-\text{Gd}} - J_{\text{Gd}-5\text{d}}) S_{\text{core}}(S_{\text{core}}+1), \tag{2}$$

where $S$ is the total spin of the system and $S_{\text{core}}$ is the total spin of the Gd 4f electrons of both ions. $S_{\text{core}}$ can therefore have integer values ranging from 0 to 7 and the allowed values of $S$ are $S_{\text{core}} \pm 1/2$ for each value of $S_{\text{core}}$ except for $S_{\text{core}} = 0$ when only $S = +1/2$ is allowed.

### B. Extraction of exchange coupling constants from broken symmetry DFT calculations

Values of the exchange coupling constants in (1) can be extracted from DFT calculations using the broken symmetry (BS) formalism pioneered by Noodleman.[11–13] Energies of three Ising configurations, $|7/2, 7/2, 1/2\rangle$, $|7/2, -7/2, 1/2\rangle$ and $|7/2, 7/2, -1/2\rangle$, were calculated at unrestricted DFT level with no constraints placed on spatial or spin symmetries. The values in the kets list the effective local spin-projections of the two Gd ions and the lone 5d electron in that order. The energies of these states were interpreted as diagonal elements of

(1) acting on the respective states.[14] The energies can then be expressed as

$$E(7/2, 7/2, 1/2) = -\frac{49}{4} J_{\mathrm{Gd-Gd}} - \frac{7}{2} J_{\mathrm{Gd-5d}} \quad (3)$$

$$E(7/2, -7/2, 1/2) = \frac{49}{4} J_{\mathrm{Gd-Gd}} \quad (4)$$

$$E(7/2, 7/2, -1/2) = -\frac{49}{4} J_{\mathrm{Gd-Gd}} + \frac{7}{2} J_{\mathrm{Gd-5d}} \quad (5)$$

and the coupling constants can be evaluated as

$$J_{\mathrm{Gd-Gd}} = \frac{1}{49}[2E(7/2, -7/2, 1/2) - E(7/2, 7/2, -1/2) - E(7/2, 7/2, 1/2)] \quad (6)$$

$$J_{\mathrm{Gd-5d}} = \frac{1}{7}[E(7/2, 7/2, -1/2) - E(7/2, 7/2, 1/2)]. \quad (7)$$

The Ising states were computed for **2**, **1'** and **2'**. The two coupling constants calculated for **2** and **2'** are $J_{\mathrm{Gd-Gd}} = -2.9\,\mathrm{cm}^{-1}$, $J_{\mathrm{Gd-5d}} = 390.2\,\mathrm{cm}^{-1}$ and $J_{\mathrm{Gd-Gd}} = -1.5\,\mathrm{cm}^{-1}$, $J_{\mathrm{Gd-5d}} = 388.6\,\mathrm{cm}^{-1}$, respectively. The values show that the cage plays a very small role in the exchange mechanism. The minor deviation between the $J_{\mathrm{Gd-Gd}}$ values calculated for the caged system and the dimer indicates that the cage might affect the 4f–4f interaction by possibly providing a secondary superexchange pathway in addition to the direct Gd–Gd exchange. Nonetheless, the values calculated in the presence and absence of the cage are very similar, especially when considering the typical errors in BS DFT values of exchange coupling constants. For the **1** and **1'** systems the exchange coupling constants were only calculated for the dimer **1'** because of considerable convergence difficulties in the calculation of the BS states of **1**. Based on the similarity of results obtained for **2** and **2'**, the exchange coupling constants calculated for **1'** ($J_{\mathrm{Gd-Gd}} = -1.3\,\mathrm{cm}^{-1}$, $J_{\mathrm{Gd-5d}} = 354.2\,\mathrm{cm}^{-1}$) were taken as a good approximation to the respective coupling constants in **1**.

### C. Calculation of zero-field splitting parameters

The zero-field splitting (ZFS) parameters of the ground $S = 15/2$ multiple were calculated from the results of DFT/ROCIS calculations. The calculations provide eigenvalues and eigenvectors of a spin-orbit coupled model Hamiltonian. The eigenvalues are listed in tables S4 and S5. The ROCIS eigenvectors were projected onto the subspace spanned by the different $M_S$ components of the ground multiplet to give the vectors

$$|\psi_i\rangle = \sum_{M_S} c_{M_S i} |S M_S\rangle. \quad (8)$$

Norms of the projections are very close to one as the excited multiplets are clearly separated from the ground multiplet by $\sim 20,000\,\mathrm{cm}^{-1}$. Using the CI coefficients $\{c_{M_S i}\}$ and the eigenvalues $\{E_i\}$ obtained from the DFT/ROCIS calculations a numerical effective Hamiltonian with matrix elements

$$\langle SM_S|\hat{H}_{\mathrm{num}}|SM'_S\rangle = \sum_i E_i c_{M_S i} c^*_{M'_S i}. \tag{9}$$

was constructed. This Hamiltonian was directly compared with the crystal-field (CF) pseudo-spin Hamiltonian

$$\hat{H}_{\mathrm{CF}} = \sum_{kq} B_{kq} \frac{\hat{O}_{kq}(\tilde{\mathbf{S}})}{O_{k0}(\tilde{S})}, \tag{10}$$

where $k$ is the rank of the operators, $q = -k, \cdots, k$ is the component, $\hat{O}_{kq}(\tilde{\mathbf{S}})/O_{kq}(\tilde{S})$ are Stevens operators used in the form defined in earlier work[15] and $B_{kq}$ are the CF parameters. In the present case (i. e. no first order orbital angular momentum) the pseudo-spin $\tilde{\mathbf{S}}$ is equal to the real spin $\mathbf{S}$ of the system and therefore we will substitute $\tilde{\mathbf{S}} \rightarrow \hat{\mathbf{S}}$ and $\tilde{S} \rightarrow S$ in all subsequent expressions. The matrix elements of (10) are

$$\langle SM_S|\hat{H}_{\mathrm{CF}}|SM'_S\rangle = \sum_{kq} B_{kq} \frac{C^{SM}_{SM',kq}}{C^{SS}_{SS,k0}} \tag{11}$$

as derived earlier.[15] $C^{SM}_{SM',kq}$ and $C^{SS}_{SS,k0}$ are Clebsch-Gordan coefficients[16]. The CF parameters including all relevant ranks ($k = 2, 4, 6, 8, 10, 12, 14$) were extracted by performing a linear least-squares fit on each matrix element of the Hamiltonians (9) and (10). In the present case the CI coefficients $\{c_{M_S i}\}$, and hence the CF parameters as well, are complex. The parameters are listed in tables S2 and S3 for all operator ranks which give non-zero parameters at a meaningful accuracy. Beyond rank eight the CF parameters become comparable to numerical noise. Tables S4 and S5 lists the eigenvalues of the CF Hamiltonian with various ranks included.

In order to compare the calculated CF parameters with the experimentally measured ZFS parameters $D$ and $E$, the second rank CF parameters must be related to the elements of the second rank ZFS Hamiltonian

$$\hat{H}_{\mathrm{ZFS}} = \hat{\mathbf{S}} \cdot \mathbf{D} \cdot \hat{\mathbf{S}} = \sum_{\alpha,\beta} D_{\alpha\beta} \hat{S}_\alpha \hat{S}_\beta, \tag{12}$$

where the indices $\alpha$ and $\beta$ run over the Cartesian components $x$, $y$ and $z$. The second rank terms in the CF Hamiltonian (10) can also be expanded in terms of the Cartesian spin

operators using the relations

$$\hat{O}_{2-2}(\hat{\mathbf{S}}) = \sqrt{\frac{3}{2}}\left[\hat{S}_x^2 - \hat{S}_y^2 - i\hat{S}_x\hat{S}_y - i\hat{S}_y\hat{S}_x\right], \tag{13}$$

$$\hat{O}_{2-1}(\hat{\mathbf{S}}) = \sqrt{\frac{3}{2}}\left[\hat{S}_z\hat{S}_x + \hat{S}_x\hat{S}_z - i\hat{S}_z\hat{S}_y - i\hat{S}_y\hat{S}_z\right], \tag{14}$$

$$\hat{O}_{20}(\hat{\mathbf{S}}) = 3\hat{S}_z^2 - S(S+1), \tag{15}$$

$$\hat{O}_{21}(\hat{\mathbf{S}}) = -\sqrt{\frac{3}{2}}\left[\hat{S}_z\hat{S}_x + \hat{S}_x\hat{S}_z + i\hat{S}_z\hat{S}_y + i\hat{S}_y\hat{S}_z\right], \tag{16}$$

$$\hat{O}_{22}(\hat{\mathbf{S}}) = \sqrt{\frac{3}{2}}\left[\hat{S}_x^2 - \hat{S}_y^2 + i\hat{S}_x\hat{S}_y + i\hat{S}_y\hat{S}_x\right], \tag{17}$$

and

$$O_{20}(S) = 3S^2 - S(S+1) = 105. \tag{18}$$

Expanding both (12) and the second ranks terms in (10), equating the terms with the same Cartesian spin operators and requiring that the elements of $\mathbf{D}$ are real gives the relations:

$$D_{xx} = -\frac{2}{105}\sqrt{\frac{3}{2}}\mathrm{Re}(B_{22}), \tag{19}$$

$$D_{yy} = \frac{2}{105}\sqrt{\frac{3}{2}}\mathrm{Re}(B_{22}), \tag{20}$$

$$D_{zz} = \frac{3}{105}B_{20}, \tag{21}$$

$$D_{xy} = D_{yx} = -\frac{2}{105}\sqrt{\frac{3}{2}}\mathrm{Im}(B_{22}), \tag{22}$$

$$D_{zx} = D_{xz} = \frac{2}{105}\sqrt{\frac{3}{2}}\mathrm{Re}(B_{21}), \tag{23}$$

$$D_{zy} = D_{yz} = \frac{2}{105}\sqrt{\frac{3}{2}}\mathrm{Im}(B_{21}), \tag{24}$$

where we have used the relations $B_{22} = {B_{2-2}}^*$, $\mathrm{Re}(B_{21}) = -\mathrm{Re}(B_{2-1})$ and $\mathrm{Im}(B_{21}) = \mathrm{Im}(B_{2-1})$. Once the elements of $\mathbf{D}$ have been calculated the tensor can be diagonalized to yield the three principal components $D_x$, $D_y$ and $D_z$ as the eigenvalues. The ZFS parameters $D$ and $E$ can then be defined as

$$D = D_z - \frac{1}{2}(D_x + D_y) \quad \text{and} \quad E = \frac{1}{2}(D_x - D_y). \tag{25}$$

The eigenvalues are assigned to $D_x$, $D_y$ and $D_z$ in such a way that $D_z$ is the one most clearly separated from the other values and $D_x$ and $D_y$ are chosen in such a way that the parameter $E$ is positive. For (**1**) the calculations give $D = 0.297\,\mathrm{cm}^{-1}$, $E = 0.000\,\mathrm{cm}^{-1}$ and for **2** $D = 0.375\,\mathrm{cm}^{-1}$, $E = 0.017\,\mathrm{cm}^{-1}$.

## III. DERIVATIONS

### A. Matrix elements of the free-ion Hamiltonian

We will first consider the splitting of the terms of a Gd(II) ion under the influence of SOC and Hund's rule coupling in the absence of any crystal-field. A Hamiltonian describing the low-lying spin states can be written as

$$\hat{H}_{\mathrm{Gd(II)}} = \hat{H}_{\mathrm{SOC}} + \hat{H}_{\mathrm{Hund}} = \zeta \hat{\mathbf{l}} \cdot \hat{\mathbf{s}} - J'_H \hat{\mathbf{S}}_0 \cdot \hat{\mathbf{s}}, \tag{26}$$

where $\hat{H}_{\mathrm{SOC}}$ is the spin-orbit coupling (SOC) Hamiltonian and $\hat{H}_{\mathrm{Hund}}$ is an effective Hund's rule coupling Hamiltonian which is used here in a Heisenberg-like form. The angular momentum operators $\hat{\mathbf{l}}$, $\hat{\mathbf{s}}$ and $\hat{\mathbf{S}}_0$ act on the orbital angular momentum of the 5d electron, the spin of the 5d electron and the total spin of the 4f electrons, respectively.

As a basis we use states where the seven 4f electrons form spin states $|S_0 M_0\rangle$ which are then coupled to the 5d electron represented by the state $|lm_l; sm_s\rangle$. $S_0$ is the total spin of the 4f electrons ($S_0 = 7/2$ in the present case), $M_0$ is its projection on the quantization axis, $l = 2$ and $s = 1/2$ are the orbital and spin angular momenta of the lone 5d electron, respectively, and $m_l$ and $m_s$ are the respective angular momentum projections. The quantum numbers defining the basis states are then the total spin $S$, its projection $M_S$, $S_0$, $s$, $l$ and $m_l$. Using a Clebsch-Gordan decomposition, the basis states can be expressed as

$$|S_0 s S M_S; l m_l\rangle = \sum_{m_s, M_0} |S_0 M_{S0}; l m_l; s m_s\rangle C^{S M_S}_{S_0 M_{S0}, s m_s}. \tag{27}$$

Matrix elements of $\hat{H}_{\mathrm{Hund}}$ are easy to evaluate as the bilinear term in the Hamiltonian can be expressed as $\hat{\mathbf{S}}_0 \cdot \hat{\mathbf{s}} = \frac{1}{2}(\hat{\mathbf{S}}^2 - \hat{\mathbf{S}}_0^2 - \hat{\mathbf{s}}^2)$ and the operator is diagonal with matrix elements

$$\begin{aligned} &\langle S_0 s S M_S; l m_l | \hat{H}_{\mathrm{Hund}} | S_0 s S' M'_S; l m'_l \rangle \\ &\quad = -\frac{J}{2} \left[ S(S+1) - S_0(S_0+1) - s(s+1) \right] \delta_{m_l m'_l} \delta_{SS'} \delta_{M_S M'_S}. \end{aligned} \tag{28}$$

The coupling constant $J'_H$ is used here as an effective parameter which shifts the diagonal elements of the non-Hund states to higher energy. $J'_H$ is not equal to an exchange integral.

The SOC operator can be expressed as a product of two spherical tensor operators:

$$\zeta \hat{\mathbf{l}} \cdot \hat{\mathbf{s}} = \zeta \sum_{q=-k}^{k} (-1)^q \hat{l}_q \hat{s}_{-q}, \tag{29}$$

where $k = 1$ is the rank of the operators $\hat{\mathbf{l}}$ and $\hat{\mathbf{s}}$, and

$$\hat{l}_0 = \hat{l}_z, \quad \hat{l}_{\pm 1} = \mp \frac{1}{\sqrt{2}} \left( \hat{l}_x \pm i \hat{l}_y \right) \tag{30}$$

$$\hat{s}_0 = \hat{s}_z, \quad \hat{s}_{\pm 1} = \mp \frac{1}{\sqrt{2}} \left( \hat{s}_x \pm i \hat{s}_y \right). \tag{31}$$

The matrix elements of the SOC operator between $|lm_l; sm_s\rangle$ states can be expressed by virtue of the Wigner–Eckart theorem[16] as

$$\begin{aligned}
\langle lm_l; sm_s | \hat{H}_{\text{SOC}} | lm'_l; sm'_s \rangle &= \zeta \sum_{q=-k}^{k} (-1)^q \langle lm_l; sm_s | \hat{l}_q \hat{s}_{-q} | lm'_l; sm'_s \rangle \qquad (32) \\
&= \zeta \sum_{q=-k}^{k} (-1)^q \frac{(-1)^{2(k+k)} \langle l || \hat{l}_k || l \rangle \langle s || \hat{s}_k || s \rangle}{\sqrt{(2l+1)(2s+1)}} C^{lm_l}_{lm'_l,kq} C^{sm_s}_{sm'_s,k-q} \\
&= \zeta \sum_{q=-k}^{k} (-1)^q ls \frac{C^{lm_l}_{lm'_l,kq} C^{sm_s}_{sm'_s,k-q}}{C^{ll}_{ll,k0} C^{ss}_{ss,k0}},
\end{aligned}$$

where $\langle l || \hat{l}_k || l \rangle$ and $\langle s || \hat{s}_k || s \rangle$ are reduced matrix elements which can be calculated as

$$\langle l || \hat{l}_k || l \rangle = (-1)^{2k} \frac{l\sqrt{2l+1}}{C^{ll}_{ll,k0}} \text{ and } \langle s || \hat{s}_k || s \rangle = (-1)^{2k} \frac{s\sqrt{2s+1}}{C^{ss}_{ss,k0}}. \tag{33}$$

in the case when we set $q = 0$. The final SOC matrix element between two basis states can then be obtained using the expansion in (27) as

$$\begin{aligned}
&\langle S_0 s S M_S; lm_l | \hat{H}_{\text{SOC}} | S_0 s S' M'_S; lm'_l \rangle \qquad (34) \\
&\quad = \zeta \sum_{m_s, m'_s} \sum_{M_{S0}, M'_{S0}} \langle S_0 M_{S0} | S_0 M'_{S0} \rangle \langle lm_l; sm_s | \hat{H}_{\text{SOC}} | lm'_l; sm'_s \rangle C^{SM}_{S_0 M_{S0}, sm} C^{S'M'_S}_{S_0 M'_{S0}, sm'_s} \\
&\quad = \frac{\zeta ls}{C^{ll}_{ll,k0} C^{ss}_{ss,k0}} \sum_{m_s, m'_s} \sum_{M_{S0}} \sum_q (-1)^q C^{SM_S}_{S_0 M_{S0}, sm_s} C^{S'M'_S}_{S_0 M_{S0}, sm'_s} C^{lm_l}_{lm'_l, kq} C^{sm_s}_{sm'_s, k-q} \\
&\quad = \frac{\zeta ls}{\frac{l}{\sqrt{l(l+1)}} \frac{s}{\sqrt{s(s+1)}}} \sum_{m_s, m'_s} \sum_{M_{S0}} \sum_q (-1)^q C^{SM_S}_{S_0 M_{S0}, sm_s} C^{S'M'_S}_{S_0 M_{S0}, sm'_s} C^{lm_l}_{lm'_l, kq} C^{sm_s}_{sm'_s, k-q} \\
&\quad = \zeta \sqrt{l(l+1)s(s+1)} \sum_{m_s, m'_s} \sum_{M_{S0}} \sum_q (-1)^q C^{SM_S}_{S_0 M_{S0}, sm} C^{S'M'_S}_{S_0 M_{S0}, sm'_s} C^{lm_l}_{lm'_l, kq} C^{sm_s}_{sm'_s, k-q},
\end{aligned}$$

where we have evaluated the Clebsch-Gordan coefficients in front of the summation by using the fact that $k = 1$ and the identity

$$C^{jm}_{jm,10} = \frac{m}{\sqrt{j(j+1)}}. \tag{35}$$

## B. Matrix elements of the single-ion Hamiltonians for a 4f$^7$5d$^1$ configuration

We will consider next the splitting of the Gd(II) free ion states due to the crystal field. The single-ion Hamiltonians for the Gd(II) ions within a $[Gd_2]^{5+}$ moiety are of the form

$$\begin{aligned}\hat{H}^a_{\mathrm{Hund}} + \hat{H}^a_{\mathrm{SOC}} &= \zeta \hat{\mathbf{l}} \cdot \hat{\mathbf{s}} - J'_H \hat{\mathbf{S}}_{0,a} \cdot \hat{\mathbf{s}} \\ \hat{H}^b_{\mathrm{Hund}} + \hat{H}^b_{\mathrm{SOC}} &= \zeta \hat{\mathbf{l}} \cdot \hat{\mathbf{s}} - J'_H \hat{\mathbf{S}}_{0,b} \cdot \hat{\mathbf{s}},\end{aligned} \tag{36}$$

where the indexes $a$ and $b$ refer to Gd ions housing the 5d electron, and the angular momentum operators have the same meaning as in (26).

We assume here that the crystal-field splitting is strong enough so that mixing of the $m_l = 0$ states into the $m_l = \pm 1$ states and $m_l = \pm 1$ into $m_l = \pm 2$ states by SOC can be neglected. The single-ion parts of the Hamiltonian can then be diagonalized in a basis spanned by the crystal-field orbital doublets. The single-ion Hamiltonians at ion $a$ can be written in terms of partially coupled states where the $S_{0,a}$ total spin of the 4f electrons is coupled into the 5d electron spin $s$ to give an intermediate spin $K$. The angular momentum and the 4f spin of ion $b$, $S_{0,b}$ will not be coupled in the basis states. For site $b$, the electron spin is coupled to the 4f spin $S_{0,b}$ and the spin $S_{0,a}$ is kept uncoupled. Using a Clebsch-Gordan expansion the basis states can be expressed as

$$\begin{aligned}|S_{0,a} s K M_K; a, l m_l; S_{0,b} M_{0,b}\rangle &= \sum_{M_{0,a}, m_s} |S_{0,a} M_{0,a}; a, s m_s, l m_l; S_{0,b} M_{0,b}\rangle C^{K M_K}_{S_{0,a} M_{0,a}, s m_s} \\ |S_{0,a} M_{0,a}; b, l m_l; S_{0,a} s K M_K\rangle &= \sum_{M_{0,b}, m_s} |S_{0,a} M_{0,a}; b, s m_s, l m_l; S_{0,b} M_{0,b}\rangle C^{K M_K}_{s m_s, S_{0,b} M_{0,b}},\end{aligned} \tag{37}$$

where $M_{0,a}$, $M_{0,b}$ and $M_K$ are the projections of $S_{0,a}$, $S_{0,b}$ and $K$, respectively. Technically $K$ and $M_K$ should also be indexed with $a$ or $b$ but in the present case there is no chance of confusion.

As in the case of a single ion, the Hund's rule coupling operator is diagonal:

$$\begin{aligned}&\langle S_{0,a} s K M_K; a, l m_l; S_{0,b} M_{0,b} | \hat{H}_{\mathrm{Hund}} | S_{0,a} s K' M'_K; a, l m_l; S_{0,b} M'_{0,b}\rangle \\ &\quad = -\frac{J}{2}\left[K(K+1) - S_{0,a}(S_{0,a}+1) - s(s+1)\right] \delta_{KK'} \delta_{M_K M'_K} \delta_{m_l m'_l} \delta_{M_{0,b} M'_{0,b}} \\ &\langle S_{0,a} M_{0,a}; b, l m_l; S_{0,a} s K M_K | \hat{H}_{\mathrm{Hund}} | S_{0,a} M'_{0,a}; b, l m_l; S_{0,a} s K' M'_K\rangle \\ &\quad = -\frac{J}{2}\left[K(K+1) - S_{0,b}(S_{0,b}+1) - s(s+1)\right] \delta_{KK'} \delta_{M_K M'_K} \delta_{m_l m'_l} \delta_{M_{0,a} M'_{0,a}}\end{aligned} \tag{38}$$

Following the same derivation as in equation (32), the SOC matrix elements between the 5d electron states can be expressed as

$$\langle a, lm_l, sm_s|\hat{H}_{\mathrm{SOC}}|a, lm_l', sm_s'\rangle = \zeta \sum_{q=-k}^{k} (-1)^q ls \frac{C^{lm_l}_{lm_l',kq} C^{sm_s}_{sm_s',k-q}}{C^{ll}_{ll,k0} C^{ss}_{ss,k0}}. \tag{39}$$

Within the crystal-field doublets $m_l$ and $m_l'$ are related either by $m_l = m_l'$ or by $m_l = -m_l'$. Due to the conservation of angular momentum projection, the Clebsch-Gordan coefficients in (39) give non-zero values in the $m_l = m_l'$ case only when $q = 0$ and in the case $m_l = -m_l'$ case only when $q = 2m_l$. In the present case $2m_l = \pm 2, \pm 4$ and $q = 0, \pm 1$ and therefore $q = 2m_l$ never holds. Thus, the only terms which survive the summation in (39) are the ones where $q = 0$ and $m_l = m_l'$. (39) can then be simplified using (35):

$$\langle a, lm_l, sm_s|\hat{H}_{\mathrm{SOC}}|a, lm_l', sm_s'\rangle = \zeta ls \delta_{m_l m_l'} \delta_{m_s m_s'} \frac{\frac{m_l}{\sqrt{l(l+1)}} \frac{m_s}{\sqrt{s(s+1)}}}{\frac{l}{\sqrt{l(l+1)}} \frac{s}{\sqrt{s(s+1)}}} = \zeta \delta_{m_l m_l'} \delta_{m_s m_s'} m_l m_s \tag{40}$$

and equally for ion $b$. The full matrix elements are

$$\begin{aligned} &\langle S_{0,a} sKM_K; a, lm_l; S_{0,b} M_{0,b}|\hat{H}_{\mathrm{SOC}}|S_{0,a} sK'M_K'; a, lm_l; S_{0,b} M_{0,b}'\rangle \qquad (41)\\ &\quad = \sum_{M_{0,a}, M_{0,a}'} \sum_{m_s, m_s'} \langle S_{0,a} M_{0,a}|S_{0,a} M_{0,a}'\rangle \langle S_{0,b} M_{0,b}|S_{0,b} M_{0,b}'\rangle \\ &\qquad \times \zeta \delta_{m_l m_l'} \delta_{m_s m_s'} m_l m_s C^{KM_K}_{S_{0,a} M_{0,a}, sm_s} C^{K'M_K'}_{S_{0,a} M_{0,a}', sm_s'} \\ &\quad = \delta_{m_l m_l'} \delta_{M_{0,b} M_{0,b}'} \zeta m_l \sum_{M_{0,a}, m_s} m_s C^{KM_K}_{S_{0,a} M_{0,a}, sm_s} C^{K'M_K'}_{S_{0,a} M_{0,a}, sm_s} \\ &\langle S_{0,a} M_{0,a}; b, lm_l; S_{0,a} sKM_K|\hat{H}_{\mathrm{SOC}}|S_{0,a} M_{0,a}'; b, lm_l; S_{0,a} sK'M_K'\rangle \\ &\quad = \delta_{m_l m_l'} \delta_{M_{0,a} M_{0,a}'} \zeta m_l \sum_{M_{0,b}, m_s} m_s C^{KM_K}_{sm_s, S_{0,b} M_{0,b}} C^{K'M_K'}_{sm_s, S_{0,b} M_{0,b}}. \end{aligned}$$

Because in this case the SOC operator only contains $q = 0$ components, projection of the angular momentum is conserved in the operations. It is easy to see from (41) that the only non-zero values in the summation are the ones where $M_K = M_K'$ due to the conservation of the spin projection. Therefore, in the single-ion case, the only off-diagonal elements in the SOC operator are those between same values of $M_K$ in the Hund and non-Hund states and the single-ion Hamiltonians $\hat{H}^a_{\mathrm{Hund}} + \hat{H}^a_{SOC}$ and $\hat{H}^b_{\mathrm{Hund}} + \hat{H}^b_{SOC}$ both reduce to a block-diagonal form with simple $2 \times 2$ blocks. For site $a$ these blocks are

$$\begin{bmatrix} -J_H' S_0 s + \frac{2\zeta m_l s M_K}{2S_0 + 1} & -\frac{2\zeta m_l s}{2S_0 + 1} \sqrt{(S_0 + s)^2 - {M_K}^2} \\ -\frac{2\zeta m_l s}{2S_0 + 1} \sqrt{(S_0 + s)^2 - {M_K}^2} & J_H'(S_0 s + s) - \frac{2\zeta m_l s M_K}{2S_0 + 1} \end{bmatrix}, \tag{42}$$

where we have only considered the case where $s = 1/2$ and $S_{0,a} = S_{0,b} \equiv S_0$ and have used the following table-definitions of Clebsch-Gordan coefficients for the case of $s = 1/2$:

$$
\begin{aligned}
C^{(S_0+s)M_K}_{S_0(M_K-s),ss} &= \sqrt{\frac{S_0 + M_K + s}{2S_0 + 1}} \\
C^{(S_0+s)M_K}_{S_0(M_K+s),s-s} &= \sqrt{\frac{S_0 - M_K + s}{2S_0 + 1}} \\
C^{(S_0-s)M_K}_{S_0(M_K-s),ss} &= -\sqrt{\frac{S_0 - M_K + s}{2S_0 + 1}} \\
C^{(S_0-s)M_K}_{S_0(M_K+s),s-s} &= \sqrt{\frac{S_0 + M_K + s}{2S_0 + 1}}
\end{aligned}
\tag{43}
$$

as well as the identity

$$
C^{KM_K}_{sm_s,S_0M_0} = (-1)^{s+S_0-K} C^{KM_K}_{S_0M_0,sm_s}. \tag{44}
$$

For site $b$ the signs of the off-diagonal elements are inverted. These $2 \times 2$ matrices can be easily diagonalized to give the energies of the single-ion states:

$$
\begin{aligned}
&E_{\pm}(J'_H, \zeta; S_0, M_K, m_l) \\
&= \frac{1}{2} J'_H \pm \frac{1}{2} \sqrt{J'^2_H s^2 (2S_0 + 1)^2 - 8J'_H \zeta m_l s^2 M_K + \zeta^2 m_l^2 \frac{16 s^2 (S_0 + s)}{(2S_0 + 1)^2}}.
\end{aligned}
\tag{45}
$$

In the case of $J'_H \to \infty$, there is no coupling between the Hund and non-Hund states. At this limit it is immediately clear from (42) that the single-ion Hamiltonian is diagonal with eigenvalues

$$
E_{J'_H \to \infty}(\zeta; M_K, m_l) = \pm \frac{2\zeta m_l s M_K}{2S_0 + 1}, \tag{46}
$$

where Hund and non-Hund states have a positive and negative sign, respectively.

## C. Matrix elements of the transfer Hamiltonian for $\Pi$ and $\Delta$ 5d states

Next we will consider the interaction between the Gd ions in the $[Gd_2]^{5+}$ moiety due to electron delocalization, or in other words, under transfer interaction. In this subsection we will consider the case where the "extra" electron occupies a 5d orbital. The spatial extent of the 5d orbitals is much larger than that of the 4f orbitals and therefore the crystal field

splitting of the 5d manifold is strong. On the other hand, the SOC constant of the 5d orbitals is weaker than that of the 4f orbitals and therefore we will assume that the crystal-field splitting is the dominant interaction and the crystal field states characterized by the quantum number $M_K$ are split and mixed by the SOC.

The transfer Hamiltonian mixing the single-ion states is of the form

$$\hat{H}_{\text{transfer}} = \sum_{m_l'',m_s''} t_{m_l''} \left[ \hat{a}^\dagger_{m_l'',m_s''} \hat{b}_{m_l'',m_s''} + \hat{b}^\dagger_{m_l'',m_s''} \hat{a}_{m_l'',m_s''} \right], \tag{47}$$

where $\hat{a}^\dagger_{m_l,m_s}$ ($\hat{a}_{m_l,m_s}$) creates (annihilates) an electron with spin projection $m_s$ into an orbital with angular momentum projection $m_l$ at ion $a$. $\hat{b}_{m_l,m_s}$ and $\hat{b}^\dagger_{m_l,m_s}$ act accordingly at ion $b$. The 5d electron states can be expressed as

$$|a, sm_s, lm_l\rangle = \hat{a}^\dagger_{m_l,m_s}|5\text{d}^0\rangle \quad \text{and} \quad |b, sm_s, lm_l\rangle = \hat{b}^\dagger_{m_l,m_s}|5\text{d}^0\rangle, \tag{48}$$

where $|5\text{d}^0\rangle$ is an empty 5d orbital space (i. e. a null vector in the Fock space of the 5d orbital states). Using these relations, matrix elements of $\hat{H}_{\text{transfer}}$ between 5d states can be expressed as

$$\begin{aligned}\langle a, sm_s, lm_l|\hat{H}_{\text{transfer}}|b, sm_s', lm_l'\rangle = \sum_{m_l'',m_s''} t_{m_l''} \Big[ &\langle 5\text{d}^0|\hat{a}_{m_l,m_s}\hat{a}^\dagger_{m_l'',m_s''}\hat{b}_{m_l'',m_s''}\hat{b}^\dagger_{m_l',m_s'}|5\text{d}^0\rangle \\ &+ \langle 5\text{d}^0|\hat{a}_{m_l,m_s}\hat{b}^\dagger_{m_l'',m_s''}\hat{a}_{m_l'',m_s''}\hat{b}^\dagger_{m_l',m_s'}|5\text{d}^0\rangle \Big] \\ =& \delta_{m_l m_l'}\delta_{m_s m_s'} t_{m_l}\end{aligned} \tag{49}$$

and the full matrix element as

$$\begin{aligned}&\langle S_{0,a} sKM_K; a, lm_l; S_{0,b}M_{0,b}|\hat{H}_{\text{transfer}}|S_{0,a}M_{0,a}'; b, lm_l; S_{0,a}sK'M_K'\rangle \\ &\quad = \sum_{M_{0,a},M_{0,b}'} \sum_{m_s,m_s'} \langle S_{0,a}M_{0,a}|S_{0,a}M_{0,a}'\rangle\langle S_{0,b}M_{0,b}|S_{0,b}M_{0,b}'\rangle \\ &\quad\quad \times \langle a, sm_s, lm_l|\hat{H}_{\text{transfer}}|b, sm_s', lm_l'\rangle C^{KM_K}_{S_{0,a}M_{0,a},sm_s} C^{K'M_K'}_{sm_s',S_{0,b}M_{0,b}'} \\ &\quad = \delta_{m_l m_l'} t_{m_l} \sum_{m_s} C^{KM_K}_{S_{0,a}M_{0,a}',sm_s} C^{K'M_K'}_{sm_s,S_{0,b}M_{0,b}}.\end{aligned} \tag{50}$$

$\hat{H}_{\text{full}} = \hat{H}^a_{\text{Hund}} + \hat{H}^a_{\text{SOC}} + \hat{H}^b_{\text{Hund}} + \hat{H}^b_{\text{SOC}} + \hat{H}_{\text{transfer}}$ will be block-diagonal in blocks corresponding to the same values of $M_K + M_{0,b}$ or $M_K' + M_{0,a}'$ and $m_l$. Size of the blocks vary from $2 \times 2$ in the case of $M_K + M_{0,b} = M_K' + M_{0,a}' = \pm 15/2$ to $30 \times 30$ in the case of $M_K + M_{0,b} = M_K' + M_{0,a}' = \pm 1/2$. With the exception of the $2 \times 2$ blocks, no analytical

form can be given for the eigenvalues and $\hat{H}_{\text{full}}$ can only be diagonalized numerically. This is also the case if we let $J'_H \to \infty$. In the case $t \ll \zeta$, $J'_H \to \infty$ all mixing between the different single-ion states characterized by different quantum numbers $M_K$ can be neglected. At this limit $\hat{H}_{\text{transfer}}$ can be exactly diagonalized in each subspace corresponding to a given value of $M_K = M'_K$. Conservation of the angular momentum projection also implies that $M_{0,b} = M'_{0,a} \equiv M_0$ and $m_l = m'_l$. Splitting of the single-ion states is then given as

$$E_{\pm}(t; K, M_K, M_0) = \begin{cases} \pm\dfrac{t}{2S_0+1}\left(K + M_K\right) \text{ if } & M_0 = M_K - s \\ \pm\dfrac{t}{2S_0+1}\left(K - M_K\right) \text{ if } & M_0 = M_K + s \\ 0 \text{ else,} & \end{cases} \tag{51}$$

where we have used (50) and (43). Including also the splitting due to SOC (equation (46)) gives

$$E_{\pm}(t; K, M_K, M_0, m_l) = \begin{cases} \dfrac{2\zeta m_l s M_K \pm t\left(K + M_K\right)}{2S_0+1} & \text{if} \quad M_0 = M_K - s \\ \dfrac{2\zeta m_l s M_K \pm t\left(K - M_K\right)}{2S_0+1} & \text{if} \quad M_0 = M_K + s \\ \dfrac{2\zeta m_l s M_K}{2S_0+1} & \text{else.} \end{cases} \tag{52}$$

This result is equivalent to the first order perturbation correction to the single-ion states due to the transfer interaction.

## D. Matrix elements of the transfer Hamiltonian for 4f configurations

The other case of electron delocalization we will consider here is the situation where the "extra" electron occupies a 4f orbital and the 5d shell is empty. As opposed to the $4f^7 5d^1$ case, this time SOC is very strong and crystal-field splitting is weaker due to the contracted nature of the 4f orbitals. Therefore SOC is the dominant interaction and we will first couple the orbital momentum to the total spins at the individual ions which, assuming that the system has an approximate axial symmetry, results into a single ion state characterized by total angular momentum $J_0$ and its projection $M_{J0}$. These states are first split by the crystal field and then by the transfer interaction. Again, due to the contracted nature of the 4f orbitals the transfer interaction is very weak as is evident from the small values of the transfer parameters listed in tables S6 and S7.

In the present case the 4f shell is more than half-filled and, thus, following Hund's rules $J_0 = K + l$, where $K$ is the total spin at the ion. We will only consider the lowest Hund's configuration and thus $K = 3$, $l = 3$ and $J_0 = 6$. Each state with the same absolute projection $|M_{J0}|$ is degenerate and we will assume that the splitting between the $\pm M_{J0}$ doublets is strong enough to neglect any mixing between them by the transfer interaction. The basis states for the diagonalization of the transfer Hamiltonian are then defined as

$$|alKJ_0M_{J0}; S_{0,b}M_{0,b}\rangle = \sum_{M_{0,a}} \sum_{m_l,m_s} \sum_{M_K} |S_{0,a}M_{0,a}; a, sm_s, lm_l; S_{0,b}M_{0,b}\rangle C^{KM_K}_{S_{0,a}M_{0,a},sm_s} C^{J_0M_{J0}}_{KM_K,lm_l} \tag{53}$$

$$|S_{0,a}M'_{0,a}; blKJ'_0M'_{J0}\rangle = \sum_{M'_{0,b}} \sum_{m'_l,m'_s} \sum_{M'_K} |S_{0,a}M'_{0,a}; b, sm'_s, lm'_l; S_{0,b}M'_{0,b}\rangle C^{KM'_K}_{sm'_s,S_{0,b}M'_{0,b}} C^{J_0M'_{J0}}_{lm'_l,KM'_K},$$

where we have followed the $LS$ coupling scheme by first coupling the spin of the "extra" 4f electron, $s$, into the total spin $S_0$ of the other 4f electrons at the same ion to form the intermediate spin $K$ and this spin is then coupled to the orbital angular momentum at that ion. As the "extra" electron is the only source of orbital momentum the total one-site angular momentum equals the orbital momentum of the "extra" electron, $l$.

A matrix element of the transfer Hamiltonian (47) between the basis states can be calculated using (49) as

$$\langle alKJ_0M_{J0}; S_{0,b}M_{0,b}|\hat{H}_{\text{transfer}}|S_{0,a}M_{0,a}; blKJ'_0M'_{J0}\rangle = \sum_{m_l,m_s} \sum_{M_K,M'_K} t_{m_l} C^{KM_K}_{S_{0,a}M'_{0,a},sm_s} C^{J_0M_{J0}}_{KM_K,lm_l} C^{KM'_K}_{sm_s,S_{0,b}M_{0,b}} C^{J_0M'_{J0}}_{lm'_l,KM'_K}. \tag{54}$$

The Clebsch-Gordan coefficients imply the following conservation rules for the angular momentum projections:

$$M'_{0,a} - M_{0,b} = M_K - M'_K = M_{J0} - M'_{J0}. \tag{55}$$

If $M_{J0} = M'_{J0}$ then it follows from (55) that $M'_{0,a} = M_{0,b} \equiv M_0$ and $M_K = M'_K$. If $M_{J0} = -M'_{0,J}$, then $M'_{0,a} - M_{0,b} = 2M_{J0}$ which in the present case ($S'_{0,a} = S_{0,b} = 7/2$ and $M_{J0}$ is integer) holds only when $0 < |M_{J0}| \leq 3$. In other words, for $|M_{J0}|$ values zero or greater than three, one only needs to consider matrix elements between states $M_{J0} = M'_{J0}$. In this case, $\hat{H}_{\text{transfer}}$ becomes block-diagonal with $2\times 2$ blocks with each block corresponding

to a different pair of values of $M_0$ and $M_{J0}$. The corresponding eigenvalues are

$$E_{\pm}(\{t_{m_l}\};J_0, M_{J0}, K, S_0, M_0) \tag{56}$$
$$= \pm \sum_{m_l} t_{m_l} \left[ \left( C^{J_0 M_{J0}}_{K(M_0-s),lm_l} \right)^2 \frac{S_0 + M_0}{2S_0 + 1} - \left( C^{J_0 M_{J0}}_{K(M_0+s),lm_l} \right)^2 \frac{S_0 - M_0}{2S_0 + 1} \right],$$

where we have again only considered the case when $s = 1/2$. For the case $0 < |M_{J0}| \leq 3$ the blocks in $\hat{H}_{\text{transfer}}$ become increasingly larger for smaller values of $|M_J|$. In the present case the Hamiltonian can still be analytically diagonalized but no useful general expression for the eigenvalues can be formulated. The eigenvalues are listed in Table (S8).

## IV. ADDITIONAL FIGURES

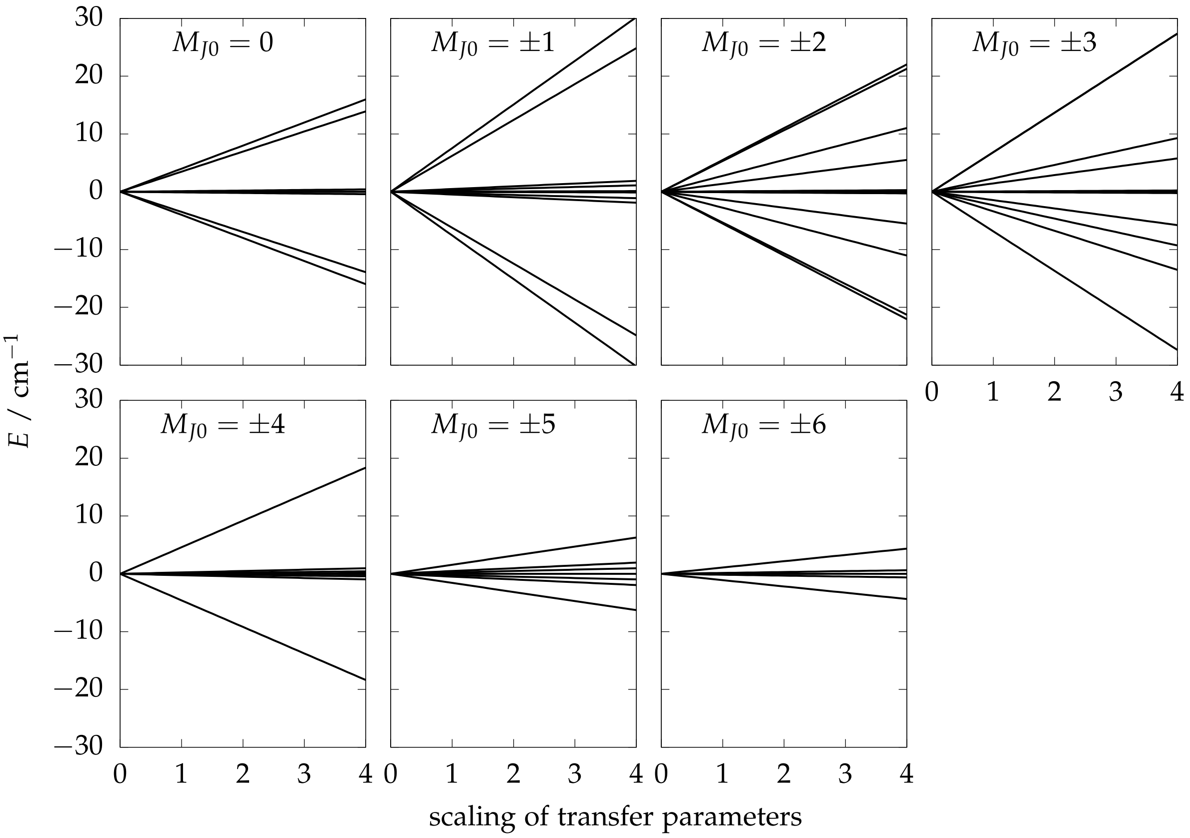


FIG. S1. Splitting of $M_{J0}$ doublets in **1** by transfer interaction when the "extra" electron is in a 4f orbital. The numbers on the horizontal axis indicate uniform scaling of the four $t_{|m_l|}$ parameters (i.e. a value of one indicates the *ab initio* calculated values). The splitting in **2** is very similar.

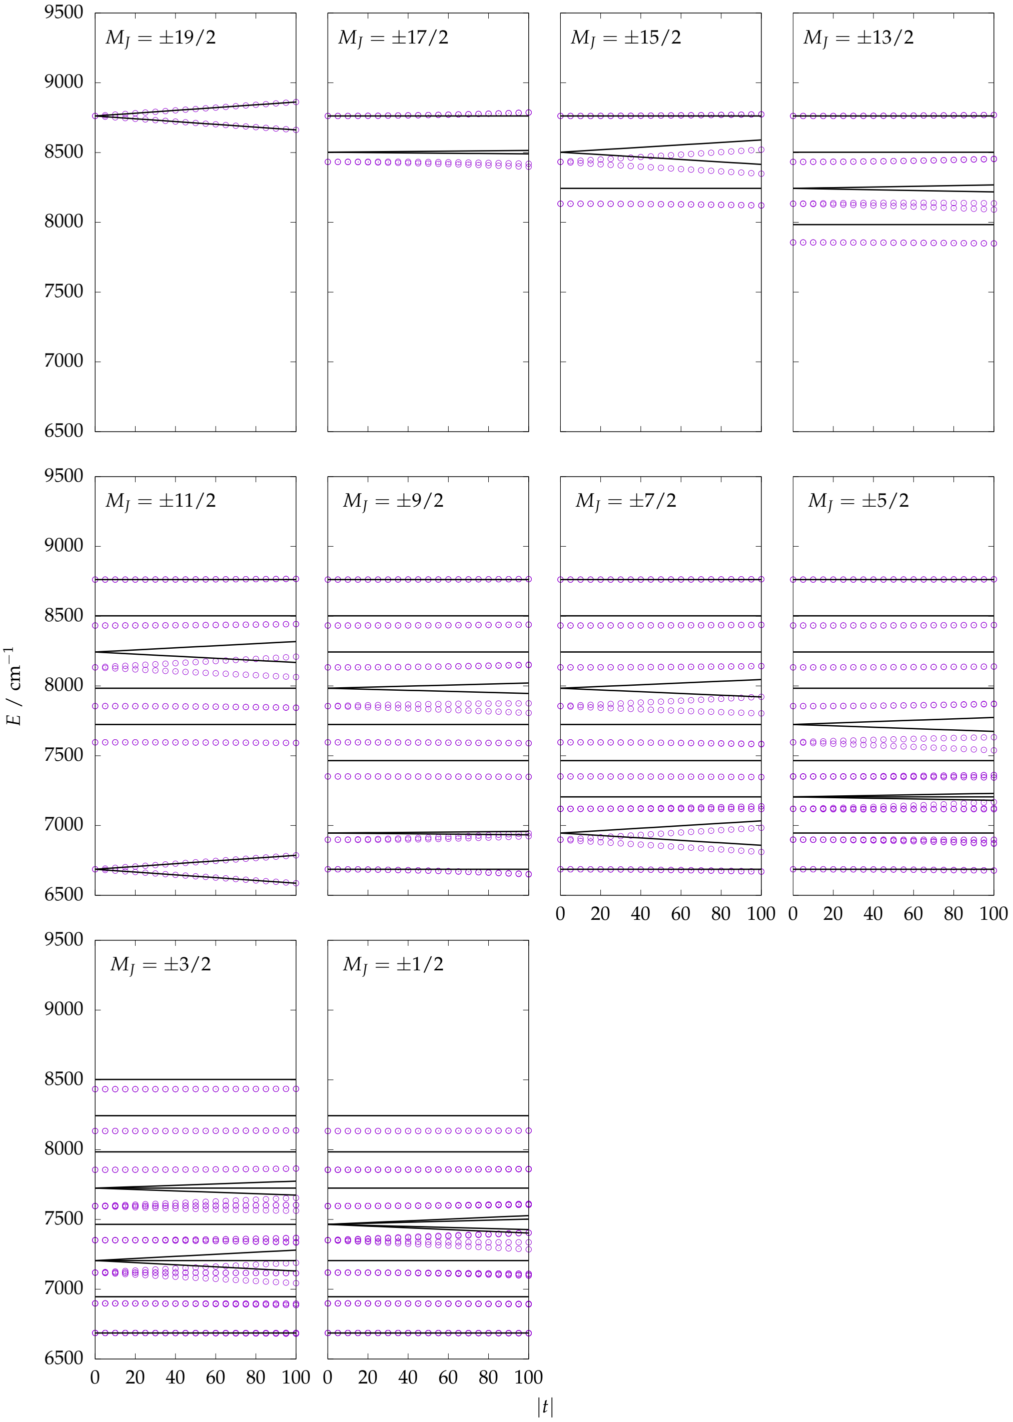


FIG. S2. Comparison of the transfer-split $\Delta$ states in the Hund manifold of **1** as calculated by numerical diagonalization of the full Hamiltonian (circles) or by the approximate equation (52) (solid lines). Mixing between Hund and non-Hund single-ion states by SOC has been neglected. The splitting in **2** is very similar.

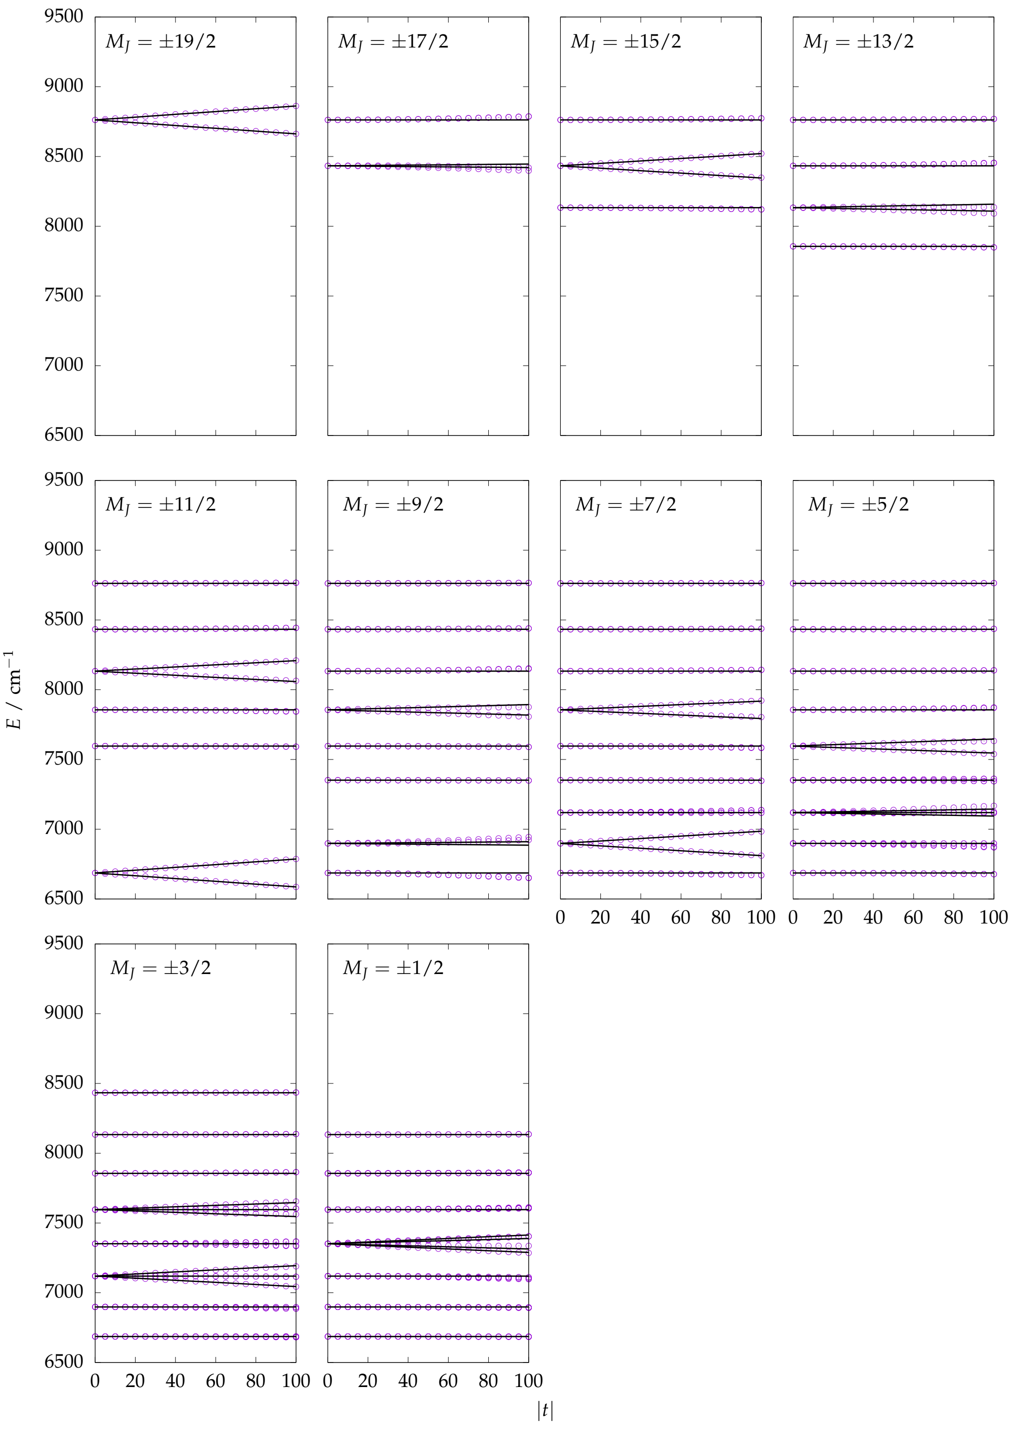


FIG. S3. Comparison of the transfer-split $\Delta$ states in the Hund manifold of **1** as calculated by numerical diagonalization of the full Hamiltonian (circles) or by the approximate equation (51) (solid lines). Mixing between Hund and non-Hund states has been included in the single-ion energies using equation (45) and the splitting of these energies has been calculated using (51). The splitting in **2** is very similar.

## V. ADDITIONAL TABLES

TABLE S1. Energies (in $cm^{-1}$) of the spin states in the exchange manifolds arising from the ground $\Sigma$ terms of **1** and **2** as calculated from exchange coupling constants extracted from broken symmetry (BS) DFT calculations and energies obtained at CASSCF level ($S_{\text{core}}$ is the total spin of the 4f electron of the two ions added together)

| | | BS DFT | | CASSCF | |
|---|---|---|---|---|---|
| $S_{\text{core}}$ | $S$ | **1** | **2** | **1** | **2** |
| 7 | 15/2 | 0 | 0 | 0 | 0 |
| 6 | 13/2 | 168 | 184 | 323 | 361 |
| 5 | 11/2 | 337 | 369 | 513 | 575 |
| 4 | 9/2 | 508 | 556 | 704 | 789 |
| 3 | 7/2 | 680 | 745 | 895 | 1003 |
| 2 | 5/2 | 853 | 935 | 1086 | 1217 |
| 1 | 3/2 | 1028 | 1126 | 1276 | 1431 |
| 0 | 1/2 | 1203 | 1319 | 1467 | 1645 |
| 1 | 1/2 | 1559 | 1709 | 1848 | 2073 |
| 2 | 3/2 | 1739 | 1906 | 2039 | 2287 |
| 3 | 5/2 | 1920 | 2105 | 2229 | 2501 |
| 4 | 7/2 | 2102 | 2305 | 2420 | 2715 |
| 5 | 9/2 | 2285 | 2507 | 2610 | 2929 |
| 6 | 11/2 | 2470 | 2710 | 2801 | 3143 |
| 7 | 13/2 | 2656 | 2914 | 2991 | 3357 |

TABLE S2. Crystal-field parameters $B_{kq}$ (defined in equations (10) and (11)) of **2** for all ranks with non-zero parameters as extracted from DFT/ROCIS calculations

| | | **1** ($[Gd_2@C_{78}]^-$) | | |
|---|---|---|---|---|
| $q$ | $k=2$ | $k=4$ | $k=6$ | $k=8$ |
| $-8$ | | | | $0.000+0.000i$ |
| $-7$ | | | | $0.000+0.000i$ |
| $-6$ | | | $0.000+0.000i$ | $0.000+0.000i$ |
| $-5$ | | | $0.000+0.000i$ | $0.000+0.000i$ |
| $-4$ | | $0.000+0.000i$ | $0.000+0.000i$ | $0.000+0.000i$ |
| $-3$ | | $0.000+0.000i$ | $0.000+0.000i$ | $0.000+0.000i$ |
| $-2$ | $0.000+0.000i$ | $0.000+0.000i$ | $0.000+0.000i$ | $0.000+0.000i$ |
| $-1$ | $0.000+0.000i$ | $0.000+0.000i$ | $0.000+0.000i$ | $0.000+0.000i$ |
| 0 | $10.405+0.000i$ | $0.003+0.000i$ | $0.000+0.000i$ | $0.000+0.000i$ |
| 1 | $0.000+0.000i$ | $0.000+0.000i$ | $0.000+0.000i$ | $0.000+0.000i$ |
| 2 | $0.000+0.000i$ | $0.000+0.000i$ | $0.000+0.000i$ | $0.000+0.000i$ |
| 3 | | $0.000+0.000i$ | $0.000+0.000i$ | $0.000+0.000i$ |
| 4 | | $0.000+0.000i$ | $0.000+0.000i$ | $0.000+0.000i$ |
| 5 | | | $0.000+0.000i$ | $0.000+0.000i$ |
| 6 | | | $0.000+0.000i$ | $0.000+0.000i$ |
| 7 | | | | $0.000+0.000i$ |
| 8 | | | | $0.000+0.000i$ |

TABLE S3. Crystal-field parameters $B_{kq}$ (defined in equations (10) and (11)) of **2** for all ranks with non-zero parameters as extracted from DFT/ROCIS calculations

| | | **2** ($[Gd_2@C_{80}]^-$) | | |
|---|---|---|---|---|
| $q$ | $k=2$ | $k=4$ | $k=6$ | $k=8$ |
| $-8$ | | | | $0.000+0.000i$ |
| $-7$ | | | | $0.001+0.001i$ |
| $-6$ | | | $0.003+0.000i$ | $-0.002+0.000i$ |
| $-5$ | | | $-0.003+0.006i$ | $0.002-0.003i$ |
| $-4$ | | $0.028+0.042i$ | $-0.003-0.005i$ | $-0.002-0.003i$ |
| $-3$ | | $-0.002+0.003i$ | $0.003-0.002i$ | $-0.002+0.001i$ |
| $-2$ | $-0.350+0.660i$ | $0.124-0.235i$ | $0.004-0.007i$ | $-0.015+0.029i$ |
| $-1$ | $0.004+0.006i$ | $-0.005-0.007i$ | $0.002+0.003i$ | $0.000+0.000i$ |
| 0 | $13.122+0.000i$ | $0.032+0.000i$ | $-0.006+0.000i$ | $0.000+0.000i$ |
| 1 | $-0.004+0.006i$ | $0.005-0.007i$ | $-0.002+0.003i$ | $0.000+0.000i$ |
| 2 | $-0.350-0.660i$ | $0.124+0.235i$ | $0.004+0.007i$ | $-0.015-0.029i$ |
| 3 | | $0.002+0.003i$ | $-0.003-0.002i$ | $0.002+0.001i$ |
| 4 | | $0.028-0.042i$ | $-0.003+0.005i$ | $-0.002+0.003i$ |
| 5 | | | $0.003+0.006i$ | $-0.002-0.003i$ |
| 6 | | | $0.003+0.000i$ | $-0.002+0.000i$ |
| 7 | | | | $-0.001+0.001i$ |
| 8 | | | | $0.000+0.000i$ |

TABLE S4. Splitting of the ground $S = 15/2$ multiplet in **1** due to ZFS (in $cm^{-1}$) as calculated by DFT/ROCIS and by diagonalization of the CF Hamiltonian (10) with increasing number of ranks $k$ of the operators $\hat{O}_{kq}(\mathbf{S})$ included in the summation

| | | **1** ($[Gd_2@C_{78}]^-$) | | |
|---|---|---|---|---|
| DFT/ROCIS | $k = 2$ | $k = 2, 4$ | $k = 2, 4, 6$ | $k = 2, 4, 6, 8$ |
| 0.00 | 0.00 | 0.00 | 0.00 | 0.00 |
| 0.00 | 0.00 | 0.00 | 0.00 | 0.00 |
| 0.59 | 0.60 | 0.60 | 0.60 | 0.60 |
| 0.59 | 0.60 | 0.60 | 0.60 | 0.60 |
| 1.78 | 1.78 | 1.78 | 1.78 | 1.78 |
| 1.78 | 1.78 | 1.78 | 1.78 | 1.78 |
| 3.57 | 3.57 | 3.57 | 3.57 | 3.57 |
| 3.57 | 3.57 | 3.57 | 3.57 | 3.57 |
| 5.94 | 5.95 | 5.94 | 5.94 | 5.94 |
| 5.94 | 5.95 | 5.94 | 5.94 | 5.94 |
| 8.92 | 8.92 | 8.92 | 8.92 | 8.92 |
| 8.92 | 8.92 | 8.92 | 8.92 | 8.92 |
| 12.48 | 12.49 | 12.48 | 12.48 | 12.48 |
| 12.48 | 12.49 | 12.48 | 12.48 | 12.48 |
| 16.65 | 16.65 | 16.65 | 16.65 | 16.65 |
| 16.65 | 16.65 | 16.65 | 16.65 | 16.65 |

TABLE S5. Splitting of the ground $S = 15/2$ multiplet in **2** due to ZFS (in $\mathrm{cm}^{-1}$) as calculated by DFT/ROCIS and by diagonalization of the CF Hamiltonian (10) with increasing number of ranks $k$ of the operators $\hat{O}_{kq}(\mathbf{S})$ included in the summation

| | | **2** ($[Gd_2@C_{80}]^-$) | | |
|---|---|---|---|---|
| DFT/ROCIS | $k = 2$ | $k = 2, 4$ | $k = 2, 4, 6$ | $k = 2, 4, 6, 8$ |
| 0.00 | 0.00 | 0.00 | 0.00 | 0.00 |
| 0.00 | 0.00 | 0.00 | 0.00 | 0.00 |
| 1.54 | 1.32 | 1.67 | 1.66 | 1.50 |
| 1.54 | 1.32 | 1.67 | 1.66 | 1.50 |
| 2.94 | 2.75 | 3.05 | 3.03 | 2.95 |
| 2.94 | 2.75 | 3.05 | 3.03 | 2.95 |
| 5.12 | 4.92 | 5.15 | 5.13 | 5.10 |
| 5.12 | 4.92 | 5.15 | 5.13 | 5.10 |
| 8.09 | 7.92 | 8.10 | 8.09 | 8.03 |
| 8.09 | 7.92 | 8.10 | 8.09 | 8.03 |
| 11.82 | 11.65 | 11.82 | 11.81 | 11.74 |
| 11.82 | 11.65 | 11.82 | 11.81 | 11.74 |
| 16.31 | 16.15 | 16.33 | 16.33 | 16.27 |
| 16.31 | 16.15 | 16.33 | 16.33 | 16.27 |
| 21.56 | 21.39 | 21.62 | 21.60 | 21.54 |
| 21.56 | 21.39 | 21.62 | 21.60 | 21.54 |

TABLE S6. The transfer parameters (in $cm^{-1}$) between 4f and 5d orbitals of various symmetries in **1'** as calculated at PBE0 level (4f and $\pi$ and $\delta$ 5d parameters) and DFT/ROCIS level (5d $\sigma$ parameters)

| | $4f_\delta$ | $4f_\delta$ | $4f_\phi$ | $4f_\phi$ | $4f_\pi$ | $4f_\pi$ | $4f_\sigma$ |
|---|---|---|---|---|---|---|---|
| $4f_\delta$ | 3.688 | 0.000 | 0.000 | 0.000 | 0.000 | 0.000 | 0.000 |
| $4f_\delta$ | 0.000 | 3.494 | 0.000 | 0.000 | 0.000 | 0.000 | 0.000 |
| $4f_\phi$ | 0.000 | 0.000 | 0.024 | 1.245 | 0.018 | 0.020 | 0.000 |
| $4f_\phi$ | 0.000 | 0.000 | 1.245 | 0.024 | 0.020 | 0.018 | 0.000 |
| $4f_\pi$ | 0.000 | 0.000 | 0.018 | 0.023 | 0.000 | 23.091 | 0.000 |
| $4f_\pi$ | 0.000 | 0.000 | 0.023 | 0.018 | 23.091 | 0.000 | 0.000 |
| $4f_\sigma$ | 0.000 | 0.000 | 0.000 | 0.000 | 0.000 | 0.000 | 28.213 |

| | $5d_\delta$ | $5d_\delta$ | $5d_\pi$ | $5d_\pi$ | $5d_\sigma$ |
|---|---|---|---|---|---|
| $5d_\delta$ | 268.116 | 0.000 | 0.000 | 0.000 | 0.000 |
| $5d_\delta$ | 0.000 | 268.697 | 0.000 | 0.000 | 0.000 |
| $5d_\pi$ | 0.000 | 0.000 | 2667.830 | 0.000 | 0.000 |
| $5d_\pi$ | 0.000 | 0.000 | 0.000 | 2667.830 | 0.000 |
| $5d_\sigma$ | 0.000 | 0.000 | 0.000 | 0.000 | 12557.900 |

TABLE S7. The transfer parameters (in $cm^{-1}$) between 4f and 5d orbitals of various symmetries in **2'** as calculated at PBE0 level (4f and $\pi$ and $\delta$ 5d parameters) and DFT/ROCIS level (5d $\sigma$ parameters)

| | $4f_\delta$ | $4f_\delta$ | $4f_\phi$ | $4f_\phi$ | $4f_\pi$ | $4f_\pi$ | $4f_\sigma$ |
|---|---|---|---|---|---|---|---|
| $4f_\delta$ | 6.567 | 0.000 | 0.000 | 0.000 | 0.000 | 0.000 | 0.000 |
| $4f_\delta$ | 0.000 | 6.091 | 0.000 | 0.000 | 0.000 | 0.000 | 0.000 |
| $4f_\phi$ | 0.000 | 0.000 | 0.002 | 0.247 | 0.261 | 0.057 | 0.000 |
| $4f_\phi$ | 0.000 | 0.000 | 0.247 | 0.002 | 0.057 | 0.261 | 0.000 |
| $4f_\pi$ | 0.000 | 0.000 | 0.057 | 0.256 | 40.465 | 0.072 | 0.000 |
| $4f_\pi$ | 0.000 | 0.000 | 0.256 | 0.057 | 0.072 | 40.465 | 0.000 |
| $4f_\sigma$ | 0.000 | 0.000 | 0.000 | 0.000 | 0.000 | 0.000 | 47.217 |

| | $5d_\delta$ | $5d_\delta$ | $5d_\pi$ | $5d_\pi$ | $5d_\sigma$ |
|---|---|---|---|---|---|
| $5d_\delta$ | 412.771 | 0.000 | 0.000 | 0.000 | 0.000 |
| $5d_\delta$ | 0.000 | 412.774 | 0.000 | 0.000 | 0.000 |
| $5d_\pi$ | 0.000 | 0.000 | 0.000 | 3714.974 | 0.000 |
| $5d_\pi$ | 0.000 | 0.000 | 3714.974 | 0.000 | 0.000 |
| $5d_\sigma$ | 0.000 | 0.000 | 0.000 | 0.000 | 14720.500 |

TABLE S8. Splitting of the $|M_{J0}|$ states arising from the $4f^8$ configurations on the Gd(II) ion in **1** and **2** due to 4f↔4f electron transfer

| $M_{J0} = 0$ | Exact expression | **1** / cm$^{-1}$ | **2** / cm$^{-1}$ |
|---|---|---|---|
| | $\pm\frac{25}{7392}(64t_0 + 27t_1)$ | ±8.215 | ±13.915 |
| | $\pm\frac{3}{2464}(125t_1 + 8t_2)$ | ±3.549 | ±6.220 |
| | $\pm\frac{1}{7392}(216t_2 + t_3)$ | ±0.105 | ±0.185 |
| | $\pm\frac{1}{1056}t_3$ | ±0.001 | ±0.000 |
| $M_{J0} = \pm 1$ | Exact expression | **1** / cm$^{-1}$ | **2** / cm$^{-1}$ |
| | $\pm\frac{5}{1056}\left(40t_0 + 23t_1 + \sqrt{1600t_0^2 + 860t_0t_1 + 529t_1^2}\right)$ | ±14.745 | ±25.021 |
| | $\pm\frac{1}{1056}\left(145t_1 + 23t_2 + \sqrt{21025t_1^2 + 4220t_1t_2 + 529t_2^2}\right)$ | ±6.470 | ±11.339 |
| | $\pm\frac{1}{1056}\left(40t_0 + 23t_1 - \sqrt{1600t_0^2 + 860t_0t_1 + 529t_1^2}\right)$ | ±0.971 | ±1.678 |
| | $\pm\frac{1}{1056}\left(41t_2 + t_3 + \sqrt{1681t_2^2 + 68t_2t_3 + t_3^2}\right)$ | ±0.281 | ±0.492 |
| | $\pm\frac{1}{1056}\left(145t_1 + 23t_2 - \sqrt{21025t_1^2 + 4220t_1t_2 + 529t_2^2}\right)$ | ±0.028 | ±0.050 |
| | $\pm\frac{1}{176}t_3$ | ±0.007 | ±0.005 |
| | $\pm\frac{1}{1056}\left(41t_2 + t_3 - \sqrt{1681t_2^2 + 68t_2t_3 + t_3^2}\right)$ | ±0.000 | ±0.001 |
| | 0 | 0.000 | 0.000 |
| $M_{J0} = \pm 2$ | Exact expression | **1** / cm$^{-1}$ | **2** / cm$^{-1}$ |
| | $\pm\frac{1}{132}\left(16t_0 + 19t_1 + \sqrt{256t_0^2 - 176t_0t_1 + 361t_1^2}\right)$ | ±10.764 | ±18.431 |
| | $\pm\frac{1}{132}\left(13t_1 + 8t_2 + \sqrt{169t_1^2 + 152t_1t_2 + 64t_2^2}\right)$ | ±4.929 | ±8.642 |
| | $\pm\frac{1}{132}\left(16t_0 + 19t_1 - \sqrt{256t_0^2 - 176t_0t_1 + 361t_1^2}\right)$ | ±2.723 | ±4.664 |
| | $\pm\frac{1}{264}(32t_2 + 3t_3)$ | ±0.449 | ±0.770 |
| | $\pm\frac{1}{132}\left(13t_1 + 8t_2 - \sqrt{169t_1^2 + 152t_1t_2 + 64t_2^2}\right)$ | ±0.054 | ±0.095 |
| | $\pm\frac{5}{264}t_3$ | ±0.024 | ±0.005 |
| | 0 | 0.000 | 0.000 |
| $M_{J0} = \pm 3$ | Exact expression | **1** / cm$^{-1}$ | **2** / cm$^{-1}$ |
| | $\pm\frac{1}{176}\left(8t_0 + 27t_1 + \sqrt{64t_0^2 - 324t_0t_1 + 729t_1^2}\right)$ | ±7.541 | ±13.167 |
| | $\pm\frac{9}{176}(2t_1 + 5t_2)$ | ±3.280 | ±5.757 |
| | $\pm\frac{1}{176}\left(8t_0 + 27t_1 - \sqrt{64t_0^2 - 324t_0t_1 + 729t_1^2}\right)$ | ±2.108 | ±3.542 |
| | $\pm\frac{1}{176}(27t_2 + 8t_3)$ | ±0.607 | ±0.982 |
| | $\pm\frac{1}{22}t_3$ | ±0.057 | ±0.011 |
| | 0 | 0.000 | 0.000 |
| $M_{J0} = \pm 4$ | Exact expression | **1** / cm$^{-1}$ | **2** / cm$^{-1}$ |
| | $\pm\frac{35}{176}t_1$ | ±4.592 | ±8.047 |
| | $\pm\frac{1}{176}(t_2 + 6t_3)$ | ±2.125 | ±3.739 |
| | $\pm\frac{1}{16}(t_2 + 6t_3)$ | ±0.667 | ±0.898 |
| | $\pm\frac{15}{176}t_3$ | ±0.106 | ±0.021 |
| | 0 | 0.000 | 0.000 |
| $M_{J0} = \pm 5$ | Exact expression | **1** / cm$^{-1}$ | **2** / cm$^{-1}$ |
| | $\pm\frac{7}{16}t_2$ | ±1.571 | ±2.769 |
| | $\pm\frac{1}{16}(t_2 + 6t_3)$ | ±0.691 | ±0.488 |
| | $\pm\frac{1}{8}t_3$ | ±0.156 | ±0.031 |
| | 0 | 0.000 | 0.000 |
| $M_{J0} = \pm 6$ | Exact expression | **1** / cm$^{-1}$ | **2** / cm$^{-1}$ |
| | $\pm\frac{7}{8}t_3$ | ±1.089 | ±0.216 |
| | $\pm\frac{1}{8}t_3$ | ±0.156 | ±0.031 |
| | 0 | 0.000 | 0.000 |

## VI. OPTIMIZED CARTESIAN COORDINATES OF 1 AND 2

$[Gd_2@C_{78}]^-$ (**1**):

| | $x$ / Å | $y$ / Å | $z$ / Å |
|---|---|---|---|
| C | −0.72707258 | 1.24454884 | 4.03593422 |
| C | −1.44933701 | −0.01291880 | 4.03185569 |
| C | −2.56201691 | 0.12480785 | 3.13618655 |
| C | −2.57406414 | 1.47311249 | 2.65026528 |
| C | −1.40429057 | 2.13982444 | 3.14181714 |
| C | 0.71294180 | 1.24760639 | 4.03865234 |
| C | 1.44050160 | −0.00690361 | 4.03723077 |
| C | 0.72312554 | −1.25518953 | 4.03324336 |
| C | −0.72687079 | −1.25814407 | 4.03055605 |
| C | −1.16020852 | −2.29157640 | 3.13445303 |
| C | −2.33866575 | −2.19991083 | 2.31039702 |
| C | −3.06806724 | −0.94291550 | 2.31137067 |
| C | −3.78651707 | −0.57028727 | 1.15474075 |
| C | −3.84473475 | 0.80109425 | 0.70338095 |
| C | −3.18418160 | 1.82683811 | 1.42062287 |
| C | −2.62905622 | 2.91685480 | 0.70895440 |
| C | −1.41585453 | 3.55518988 | 1.16559780 |
| C | −0.73476267 | 3.11782633 | 2.32203835 |
| C | 0.71860594 | 3.12085040 | 2.32452619 |
| C | 1.38940735 | 2.14563821 | 3.14665795 |
| C | 2.56355412 | 1.48376451 | 2.65904138 |
| C | 2.55548751 | 0.13545287 | 3.14504122 |
| C | 3.06876438 | −0.93016314 | 2.32182269 |
| C | 2.34457223 | −2.19020052 | 2.31835400 |
| C | 1.16371091 | −2.28675711 | 3.13845044 |
| C | 0.00399992 | −2.97103941 | 2.64730007 |
| C | 0.00759389 | −3.67476761 | 1.41688548 |

| | | | |
|---|---|---|---|
| C | −1.21121984 | −3.73843522 | 0.70027019 |
| C | −2.37252737 | −3.00756292 | 1.15306918 |
| C | −3.08648087 | −2.59523515 | −0.00959918 |
| C | −3.78378673 | −1.39364693 | −0.00878599 |
| C | −3.78259325 | −0.56635851 | −1.16960975 |
| C | −3.84234170 | 0.80350984 | −0.71380498 |
| C | −3.17935222 | 1.83155485 | −1.42538561 |
| C | −2.62655711 | 2.91916334 | −0.70821624 |
| C | −1.41179806 | 3.55898114 | −1.15858159 |
| C | −0.70050361 | 3.97207602 | 0.00540914 |
| C | 0.68882011 | 3.97496412 | 0.00778027 |
| C | 1.40187359 | 3.56102236 | 1.17044735 |
| C | 2.61929752 | 2.92777908 | 0.71791613 |
| C | 3.17645718 | 1.84004483 | 1.43149612 |
| C | 3.84363179 | 0.81711016 | 0.71648458 |
| C | 3.78956811 | −0.55453471 | 1.16769358 |
| C | 3.79432428 | −1.37786626 | 0.00411831 |
| C | 3.10197636 | −2.58235753 | 0.00091720 |
| C | 2.38577364 | −2.99765181 | 1.16116065 |
| C | 1.22903100 | −3.73335864 | 0.70442415 |
| C | 1.23141295 | −3.73086098 | −0.71278850 |
| C | 0.01237252 | −3.66977907 | −1.42905603 |
| C | −1.20880883 | −3.73607661 | −0.71692598 |
| C | −2.36855661 | −3.00357911 | −1.17129934 |
| C | −2.33087198 | −2.19210349 | −2.32576778 |
| C | −3.06029838 | −0.93506545 | −2.32503692 |
| C | −2.55148710 | 0.13538492 | −3.14494200 |
| C | −2.56493752 | 1.48195257 | −2.65409405 |
| C | −1.39354682 | 2.15033556 | −3.13932840 |
| C | −0.72667394 | 3.12553169 | −2.31413585 |

| | | | |
|---|---|---|---|
| C | 0.72666066 | 3.12853978 | −2.31165093 |
| C | 1.40592602 | 3.56503765 | −1.15374338 |
| C | 2.62169667 | 2.93016260 | −0.69924492 |
| C | 3.18156973 | 1.84495920 | −1.41473386 |
| C | 3.84615085 | 0.81952474 | −0.70070082 |
| C | 3.79372506 | −0.55057105 | −1.15662369 |
| C | 3.07676054 | −0.92216733 | −2.31450432 |
| C | 2.35261225 | −2.18221738 | −2.31774322 |
| C | 2.38966457 | −2.99355313 | −1.16316324 |
| C | 1.17440086 | −2.27593568 | −3.14210900 |
| C | 0.01302086 | −2.96157157 | −2.65697305 |
| C | −1.14956896 | −2.28093491 | −3.14647474 |
| C | −0.71342886 | −1.24506357 | −4.03893630 |
| C | −1.43610094 | 0.00057213 | −4.03813271 |
| C | −0.71332032 | 1.25784085 | −4.03373769 |
| C | 0.72634971 | 1.26070238 | −4.03031583 |
| C | 1.40030621 | 2.15624324 | −3.13445791 |
| C | 2.57315951 | 1.49296053 | −2.64564473 |
| C | 2.56641852 | 0.14611301 | −3.13576760 |
| C | 1.45388576 | 0.00657664 | −4.03113519 |
| C | 0.73678483 | −1.24170761 | −4.03535664 |
| Gd | 0.00000000 | 0.00000000 | −2.04384000 |
| Gd | 0.00000000 | 0.00000000 | 2.04383688 |

$[Gd_2@C_{80}]^-$ (**2**):

| | $x$ / Å | $y$ / Å | $z$ / Å |
|---|---|---|---|
| C | 1.24215990 | 0.56786851 | −3.96979570 |
| C | −0.01262376 | 1.32743327 | −3.98707706 |
| C | 0.20437784 | 2.51325502 | −3.19121711 |
| C | 2.17901984 | 1.31828030 | −3.16781222 |
| C | 1.55020776 | 2.51698230 | −2.72544752 |

| | | | |
|---|---|---|---|
| C | 3.20660279 | 0.72106301 | −2.37013660 |
| C | 3.25928008 | −0.69204910 | −2.36273458 |
| C | 1.25360493 | −0.87679944 | −3.88460942 |
| C | 2.26266422 | −1.46264932 | −3.06310734 |
| C | −0.03172290 | −1.53484711 | −3.88826615 |
| C | −1.29956562 | 0.66666193 | −3.91978797 |
| C | −1.28430349 | −0.77819773 | −3.90498037 |
| C | −2.29774774 | 1.29444934 | −3.11445219 |
| C | −0.81413588 | 3.15251242 | −2.41425084 |
| C | −2.08972357 | 2.54173553 | −2.42151368 |
| C | −0.42449267 | 3.87089794 | −1.26096204 |
| C | 1.94396527 | 3.18980255 | −1.52882188 |
| C | 0.94059193 | 3.89554545 | −0.82463875 |
| C | 3.64320082 | 1.41163511 | −1.21636049 |
| C | 3.02367476 | 2.63597971 | −0.80198247 |
| C | 4.03126606 | 0.69326983 | −0.04107331 |
| C | 3.65288642 | −1.40956174 | −1.19880728 |
| C | 3.99859862 | −0.72206358 | −0.00197940 |
| C | 2.06108422 | −2.66968352 | −2.30250350 |
| C | 2.91127986 | −2.63442777 | −1.16180625 |
| C | −0.24174245 | −2.68322795 | −3.04217399 |
| C | 0.78589656 | −3.27909779 | −2.24735359 |
| C | −2.21648947 | −1.48980191 | −3.06480193 |
| C | −1.58443443 | −2.66533275 | −2.56905014 |
| C | −3.28519906 | 0.56258389 | −2.36133859 |
| C | −3.23362976 | −0.84931802 | −2.29129656 |
| C | −2.92647565 | 2.56795803 | −1.27123785 |
| C | −3.66695419 | 1.34268123 | −1.23427241 |
| C | −1.25995168 | 3.89217715 | −0.09895888 |
| C | −2.49851975 | 3.20585553 | −0.07320710 |

| | | | |
|---|---|---|---|
| C | 0.94842774 | 3.93520464 | 0.60113648 |
| C | −0.41192341 | 3.93535398 | 1.05239100 |
| C | 3.03197130 | 2.67539051 | 0.62379709 |
| C | 3.65691506 | 1.47560200 | 1.09703995 |
| C | 1.96075646 | 3.26943645 | 1.33224021 |
| C | 3.23144946 | 0.84967231 | 2.29131106 |
| C | 3.66470117 | −1.34230563 | 1.23427409 |
| C | 3.28299124 | −0.56223481 | 2.36135905 |
| C | 2.49628901 | −3.20551307 | 0.07320926 |
| C | 2.92421636 | −2.56756925 | 1.27123014 |
| C | 0.40971489 | −3.93503650 | −1.05238217 |
| C | 1.25775251 | −3.89185767 | 0.09896096 |
| C | −1.96294870 | −3.26909956 | −1.33225539 |
| C | −0.95063952 | −3.93490598 | −0.60113433 |
| C | −3.65908171 | −1.47524724 | −1.09702240 |
| C | −3.03413989 | −2.67503620 | −0.62379496 |
| C | −4.00078560 | 0.72242198 | 0.00198645 |
| C | −4.03344442 | −0.69292658 | 0.04108412 |
| C | −2.91351189 | 2.63479565 | 1.16181087 |
| C | −3.65511214 | 1.40992502 | 1.19881189 |
| C | −0.78813307 | 3.27944727 | 2.24737649 |
| C | −2.06331675 | 2.67005634 | 2.30251614 |
| C | 1.58222161 | 2.66560513 | 2.56900145 |
| C | 2.21430587 | 1.49013848 | 3.06485417 |
| C | 0.23953469 | 2.68350726 | 3.04212783 |
| C | 1.28220446 | 0.77857221 | 3.90528160 |
| C | 0.02956265 | 1.53517473 | 3.88822989 |
| C | 2.29554291 | −1.29410819 | 3.11455800 |
| C | 2.08749832 | −2.54136965 | 2.42151971 |
| C | 1.29747728 | −0.66636885 | 3.92018823 |

| | | | |
|---|---|---|---|
| C | 0.42229309 | −3.87059907 | 1.26097243 |
| C | −0.94278908 | −3.89522904 | 0.82463101 |
| C | 0.81191412 | −3.15219270 | 2.41426419 |
| C | −3.02584132 | −2.63561413 | 0.80199075 |
| C | −3.64538911 | −1.41127896 | 1.21637632 |
| C | −1.94616975 | −3.18949935 | 1.52883652 |
| C | −3.26151579 | 0.69241903 | 2.36275990 |
| C | −2.26491802 | 1.46302523 | 3.06308757 |
| C | −1.25570364 | 0.87707092 | 3.88422464 |
| C | −3.20880439 | −0.72069297 | 2.37015676 |
| C | 0.01048054 | −1.32712304 | 3.98713035 |
| C | −0.20658380 | −2.51296935 | 3.19124956 |
| C | −1.55239500 | −2.51667359 | 2.72543791 |
| C | −1.24422191 | −0.56750079 | 3.96944858 |
| C | −2.18115938 | −1.31791874 | 3.16769852 |
| Gd | 0.00000000 | 0.00000000 | −1.93690500 |
| Gd | 0.00000000 | 0.00000016 | 1.93690269 |

## REFERENCES


[1] J. P. Perdew, K. Burke, and M. Ernzerhof, Phys. Rev. Lett. **77**, 3865 (1996).

[2] J. P. Perdew, K. Burke, and M. Ernzerhof, Phys. Rev. Lett. **78**, 1396 (1997).

[3] D. N. Laikov and Y. A. Ustynyuk, Russ. Chem. Bull. **54**, 820 (2005).

[4] B. Cao, T. Wakahara, T. Tsuchiya, M. Kondo, Y. Maeda, G. M. Aminur Rahman, T. Akasaka, K. Kobayashi, S. Nagase, and K. Yamamoto, J. Am. Chem. Soc. **126**, 9164 (2004).

[5] M. Yamada, T. Wakahara, T. Tsuchiya, Y. Maeda, M. Kako, T. Akasaka, K. Yoza, E. Horn, N. Mizorogi, and S. Nagase, Chem. Commun. , 558 (2008).

[6] M. M. Olmstead, A. de Bettencourt-Dias, J. C. Duchamp, S. Stevenson, D. Marciu, H. C. Dorn, and A. L. Balch, Angew. Chem. Int. Ed. **40**, 1223 (2001).

[7] T. Yumura, Y. Sato, K. Suenaga, and S. Iijima, J. Phys. Chem. B **109**, 20251 (2005).

[8] K. Tan and X. Lu, Chem. Commun. , 4444 (2005).

[9] F.-F. Li, N. Chen, M. Mulet-Gas, V. Triana, J. Murillo, A. Rodríguez-Fortea, J. M. Poblet, and L. Echegoyen, Chem. Sci. **4**, 3404 (2013).

[10] O. Kahn, *Molecular Magnetism* (VHC, New York, 1993).

[11] L. Noodleman, J. Chem. Phys. **74**, 5737 (1981).

[12] L. Noodleman, J. G. N. Jr., J. H. Osborne, A. Aizman, and D. A. Case, J. Am. Chem. Soc. **107**, 3418 (1985).

[13] L. Noodleman and E. R. Davidson, Chemical Physics **109**, 131 (1986).

[14] I. d. P. R. Moreira and F. Illas, Phys. Chem. Chem. Phys. **8**, 1645 (2006).

[15] N. Iwahara and L. F. Chibotaru, Phys. Rev. B **91**, 174438 (2015).

[16] D. A. Varshalovich, A. N. Moskalev, and V. K. Khersonskii, *Quantum Theory of Angular Momentum* (World Scientific Publishing, Singapore, 1988).
